# Supplementary material for: The Overlapped Radial Basis Function-Finite Difference (RBF-FD) Method: A Generalization of RBF-FD
Source: arXiv:1606.03135 source file (2017-01-02)
Supplement: Supplementary file 1 [file Appendix.tex]

\section{Algorithms for SL Advection}
\label{sec:appendix0}

\begin{algorithm}
\caption{Semi-Lagrangian Advection on the Sphere}
\label{alg:sl_alg}
\begin{algorithmic}
  \State Given: Velocity field $\vu(\vx,t)$, $\|\vx\|_2=1$.
	\State Given: Initial scalar field $q(\vx,0)$.
	\State Given: $ X = \{\vx_k\}_{k=1}^m$, $X \subset \mathbb{S}^2$.
	\State Given: final time $T$, time-step $\Delta t$.
	\State Set $Q = \lf.q(\vx,0)\rt|_X$.
	\State Set $t=0$, $j=1$, $N_T = \frac{T}{\Delta t}$.
	\While{$j < N_T$}
	  \State \textbf{Interpolate} $Q^m$ and store the interpolation coefficients.	
		\State Trace back $\vx_k$ to find departure point $\vx^d_k$, $k=1,\hdots,N$ (\textbf{trajectory reconstruction}).
		\State Set $X_d = \{\vx^d_k\}_{k=1}^m$.
		\State \textbf{Evaluate} the interpolant at $X_d$ to obtain $Q^m_d = \lf.Q\rt|_{X_d}$.	
		\State Set $Q^{n+1} = Q^m_d$.
		\State Set $t = j \Delta t$. 
		\State Set $j = j+1$.
	\EndWhile
\end{algorithmic}
\end{algorithm}

In this section, we present our algorithms for SL advection in conjunction with global, local and partition of unity RBF interpolation. First, we present the general form of the SL advection algorithm for any interpolant and trajectory reconstruction scheme. This is shown in Algorithm \ref{alg:sl_alg}.

\begin{algorithm}
\caption{Global RBF SL Advection}
\label{alg:grbf_sl}
\begin{algorithmic}
  \State Given: Velocity field $\vu(\vx,t)$, $\|\vx\|_2=1$.
	\State Given: Initial scalar field $q(\vx,0)$.
	\State Given: $ X = \{\vx_k\}_{k=1}^m$, $X \subset \mathbb{S}^2$.
	\State Given: final time $T$, time-step $\Delta t$.
	\State Set $Q = \lf.q(\vx,0)\rt|_X$.\
	\State Find $G$ so that $A_X = GG^T$.	
	\State Set $t=0$, $j=1$, $N_T = \frac{T}{\Delta t}$.
	\While{$j < N_T$}
	  \State Solve $GG^T c^m_Q = Q^m_X$ for $c^m_Q$.
		\State Solve $\frac{d\vx^{\ell}_k}{dt} = \vu$ over $[t_{m+1},t_m]$, $k=1,\hdots,N$.
		\State Set $X_d = \{\vx^{\ell}_k(t_m) \}_{k=1}^m =  \{\vx^d_k\}_{k=1}^m$.
		\State Set $Q^m_d = A_d c^m_Q$.	
		\State Set $Q^{n+1} = Q^m_d$.
		\State Set $t = j \Delta t$. 
	  \State Set $j = j+1$.		
	\EndWhile
\end{algorithmic}
\end{algorithm}

Algorithm \ref{alg:grbf_sl} details the SL advection algorithm in conjunction with global RBFs. This is a fairly straightforward algorithm, and requires very little explanation. 
\begin{algorithm}
\caption{Local RBF SL Advection}
\label{alg:lrbf_sl}
\begin{algorithmic}
  \State Given: Velocity field $\vu(\vx,t)$, $\|\vx\|_2=1$.
	\State Given: Initial scalar field $q(\vx,0)$.	
	\State Given: $ X = \{\vx_k\}_{k=1}^m$, $X \subset \mathbb{S}^2$.
	\State Given: $n$, the number of nodes in a stencil.
	\State Given: $\kappa_T$, the target condition number.
	\State Given: final time $T$, time-step $\Delta t$.
	\State Set $Q = \lf.q(\vx,0)\rt|_X$.\
	\State Build a \textbf{kd-tree} on the set $X$.
	\For {k=1,N}
	  \State Search kd-tree and build stencil $P_k$.
		\State Build and decompose $A^H_{P_k} = L_k U_k$.
		\State Find shape parameter $\ep_k$ so that $\kappa(A_{P_k}(\ep_k)) = \kappa_T$.
		\State Store $L_k$, $U_k$ and $\ep_k$.
	\EndFor
	\State Set $t=0$, $j=1$, $N_T = \frac{T}{\Delta t}$.
	\While{$j < N_T$}	  
		\State Solve $\frac{d\vx^{\ell}_k}{dt} = \vu$ over $[t_{m+1},t_m]$, $k=1,\hdots,N$.
		\State Set $X_d = \{\vx^{\ell}_k(t_m) \}_{k=1}^m =  \{\vx^d_k\}_{k=1}^m$.	
		\State For each $\vx^d_k$, find the closest node $\vx^{nn}_k$ in $X$.
		\State Set $X_{nn} = \{\vx^{nn}_k\}_{k=1}^m$.
		\For {k=1,N}
			\State Retrieve the $L_k$, $U_k$ and $\ep_k$ values for $\vx^{nn}_k$.
			\State Solve $L_k U_k c^H_k = (Q^m)^H_k$ for the coefficients $c^H_k$.
			\State Form local evaluation matrix $(A^H_d)_k$ (uses $\ep_k$).
			\State Set $(Q^m_d)_k = (A^H_d)_k c^H_k$.
		\EndFor
		\State Set $Q^{n+1} = Q^m_d$.
		\State Set $t = j \Delta t$. 
	  \State Set $j = j+1$.		
	\EndWhile
\end{algorithmic}
\end{algorithm}

Algorithm \ref{alg:lrbf_sl} describes the uses of local RBFs within the SL advection framework. This algorithm is necessarily more complicated. Here, superscript $m$ indicates time levels, while $n$ represents the number of nearest neighbors. Note that the kd-tree can be replaced with any other efficient nearest neighbor search data structure. Indeed, research into such data structures on parallel architectures is currently underway~\cite{SrivatsaParnandiShankarKirby}.

\section{Deriving new measures of dissipation and dispersion}
\label{sec:appendix1}

In this section, we follow~\cite{Takacs,Staniforth,Bonaventura} and re-derive established quantitative measures of numerical dissipation and dispersion. We then derive our improvements to these estimates. First, we define the Mean Squared Error (M.S.E) $e_{M}$ as
\begin{align}
e_M = \frac{1}{N} \sum_{k=1}^m (q_k - Q_k)^2,
\end{align}
where $Q_k$ are the samples of the numerical solution on the node set $X$, and $q_k = q(\vx_k)$ are samples of the true solution. $e_M$ can be decomposed as follows:
\begin{align}
e_M = \sigma^2(q-Q) - (\bar{q} - \bar{Q})^2,
\end{align}
where $\sigma^2$ is the variance, and $\bar{t}$ is the mean of $t$. These quantities can be used in the function sense or purely in the statistical sense. Using a simple identity, we can decompose the first term to get
\begin{align}
e_M = \sigma^2(q) + \sigma^2(Q) - 2cov(q,Q) + (\bar{q} - \bar{Q})^2,
\end{align}
where $cov(q,Q)$ is the covariance of these two quantities. Again, this can be computed in the function sense use inner products on the surface, or in the statistical sense. We can further make this more intuitive using the Pearson correlation coefficient, $\rho$, to obtain
\begin{align}
e_M = \sigma^2(q) + \sigma^2(Q) - 2\rho\sigma(q)\sigma(Q) + (\bar{q} - \bar{Q})^2,
\end{align}
where $-1 \leq \rho \leq 1$; again, $\rho$ can either be computed statistically or in the function sense using surface integrals. It is useful to regard errors in the absolute value sense, so we now use $|\rho|$ in place of $\rho$. Further simplifying, we get
\begin{align}
e_M = \underbrace{(\sigma(q) - \sigma(Q))^2 + (\bar{q} - \bar{Q})^2}_{\textit{Correlated part}} + \underbrace{2(1-|\rho|)\sigma(q)\sigma(Q)}_{\textit{Uncorrelated part}},
\end{align}
where $\sigma$ is the standard deviation. Multiplying through by $N$, we get
\begin{align}
\|q - Q\|_2^2 = N(\sigma(q) - \sigma(Q))^2 + N(\bar{q} - \bar{Q})^2 + 2N(1-|\rho|)\sigma(q)\sigma(Q).
\end{align}
Taking the square root of the above expression, we get
\begin{align}
\|q - Q\|_2 = \sqrt{N}\sqrt{(\sigma(q) - \sigma(Q))^2 + (\bar{q} - \bar{Q})^2 + 2(1-|\rho|)\sigma(q)\sigma(Q)}.
\end{align}
To separate the above into dissipation and dispersion, we now simply split the square root, turning the above equality into an inequality. Noting that each term here is either positive or zero, we get
\begin{align}
\|q - Q\|_2 < \sqrt{N}\sqrt{(\sigma(q) - \sigma(Q))^2 + (\bar{q} - \bar{Q})^2} + \sqrt{N}\sqrt{2(1-|\rho|)\sigma(q)\sigma(Q)}.
\end{align}
If we were measuring relative errors instead, we may simply divide through by the $\|q\|_2$ to get
\begin{align}
\frac{\|q - Q\|_2}{\|q\|_2} < \underbrace{\frac{\sqrt{N}}{\|q\|_2}\sqrt{(\sigma(q) - \sigma(Q))^2 + (\bar{q} - \bar{Q})^2}}_{\textit{Relative Dissipation}} + \underbrace{\frac{\sqrt{N}}{\|q\|_2}\sqrt{2(1-|\rho|)\sigma(q)\sigma(Q)}}_{\textit{Relative Dispersion}}.
\end{align}
We note that the original intuition is unchanged, despite our modifications. We still have a correlated part, and a part that measures departure from correlation. We label the former \emph{relative dissipation}, and the latter \emph{relative dispersion}. Further, in practice, we find that
\begin{align}
\frac{\|q - Q\|_2}{\|q\|_2} \approx \underbrace{\frac{\sqrt{N}}{\|q\|_2}\sqrt{(\sigma(q) - \sigma(Q))^2 + (\bar{q} - \bar{Q})^2}}_{\textit{Relative Dissipation}} + \underbrace{\frac{\sqrt{N}}{\|q\|_2}\sqrt{2(1-|\rho|)\sigma(q)\sigma(Q)}}_{\textit{Relative Dispersion}}.
\end{align}
